# Supplementary material for: Particle contact dynamics as the origin for non-integer power expansion rheology in attractive suspension networks
Source: arXiv:2104.05678 source file (2021-11-12)
Supplement: Supplementary file 1 [file SI_2ndV2.pdf]

# Supplementary Information

## for

### Particle contact dynamics as the origin for non-integer power expansion rheology in attractive suspension networks

Irene Natalia<sup>1</sup>, Randy H. Ewoldt<sup>2</sup>, Erin Koos<sup>1,\*</sup>

<sup>1</sup> KU Leuven, Soft Matter, Rheology and Technology - Department of Chemical Engineering,  
Celestijnenlaan 200f, 3001 Leuven, Belgium

<sup>2</sup> Department of Mechanical Science and Engineering, University of Illinois at Urbana-Champaign,  
Urbana, IL 61801, USA

\* E-mail: erin.koos@kuleuven.be

## List of Figures

|     |                                                                                                                               |    |
|-----|-------------------------------------------------------------------------------------------------------------------------------|----|
| S1  | Power spectrum of capillary suspensions in the pendular state. . . . .                                                        | 2  |
| S2  | Typical viscous data set for pendular state sample (NP3-silicone oil-glycerol). . . .                                         | 3  |
| S3  | All calculated $G'_{LVE}$ (red) and $G''_{LVE}$ values (blue) from capillary suspensions in the<br>pendular state. . . . .    | 4  |
| S4  | Third harmonic elastic and viscous weakly nonlinear scaling of capillary suspensions<br>in the pendular state. . . . .        | 5  |
| S5  | Fitting results from the equation 15 for pendular state samples with different con-<br>centration of secondary fluid. . . . . | 6  |
| S6  | Confocal microscope images of capillary state samples. . . . .                                                                | 8  |
| S7  | $G'$ and $G''$ from PMMA-glycerol normal suspension. . . . .                                                                  | 9  |
| S8  | All calculated $G'_{LVE}$ (red) and $G''_{LVE}$ values (blue) from capillary suspensions in the<br>capillary state. . . . .   | 10 |
| S9  | Third harmonic elastic and viscous weakly nonlinear scaling of capillary suspensions<br>in the capillary state. . . . .       | 11 |
| S10 | Fitting results of equation 15 for PMMA in glycerol with added paraffin oil samples. . .                                      | 12 |

## List of Tables

|    |                                                                                                         |    |
|----|---------------------------------------------------------------------------------------------------------|----|
| S1 | Obtained values for the fitting parameters $A$ and $\hat{\gamma}$ for samples in the pendular state. .  | 7  |
| S2 | Ratio of viscous scaling to the elastic scaling showing the average and deviation . .                   | 8  |
| S3 | Obtained values for the fitting parameters $A$ and $\hat{\gamma}$ for samples in the capillary state. . | 13 |

## Pendular state

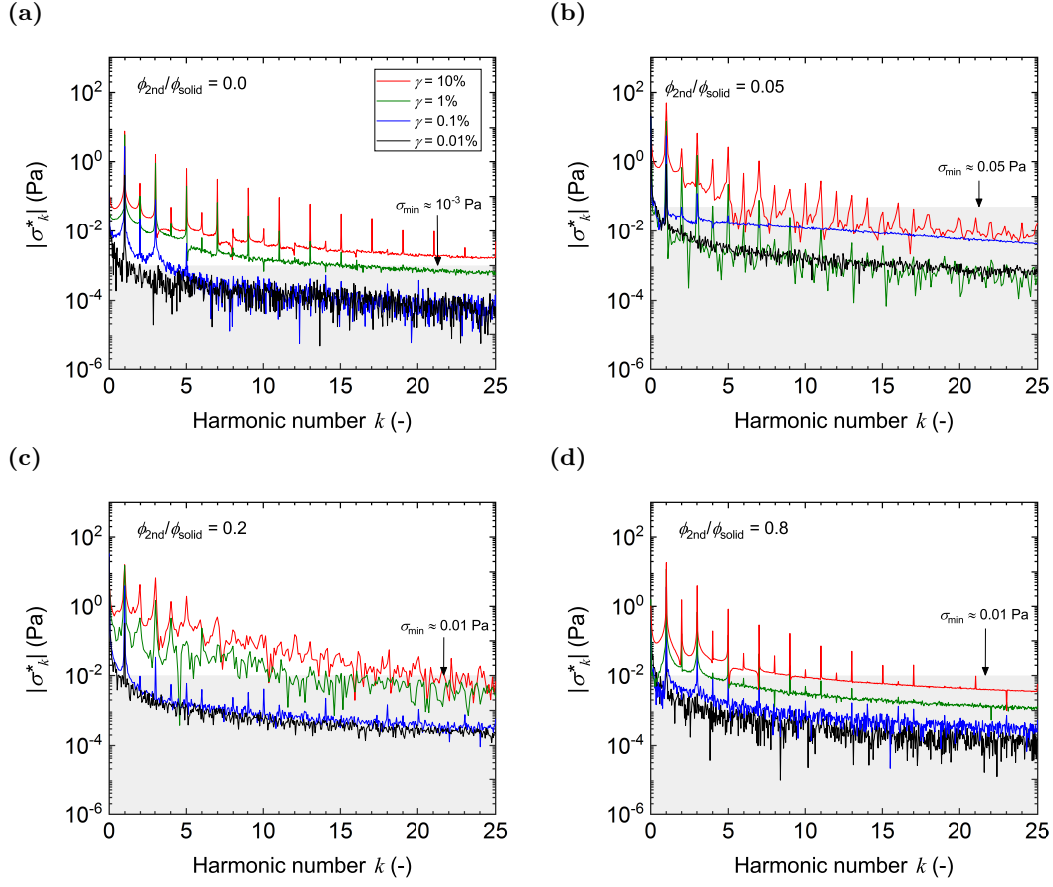

Figure S1: Power spectrum of capillary suspension in the pendular state (NP3-silicone oil-glycerol suspension) with a constant  $\phi_{\text{solid}} = 0.25$ . The gray area refers to the noise floor for each specific sample composition, where (a)  $\phi_{2\text{nd}}/\phi_{\text{solid}} = 0$ , (b)  $\phi_{2\text{nd}}/\phi_{\text{solid}} = 0.05$ , (c)  $\phi_{2\text{nd}}/\phi_{\text{solid}} = 0.2$ , and (d)  $\phi_{2\text{nd}}/\phi_{\text{solid}} = 0.8$ .

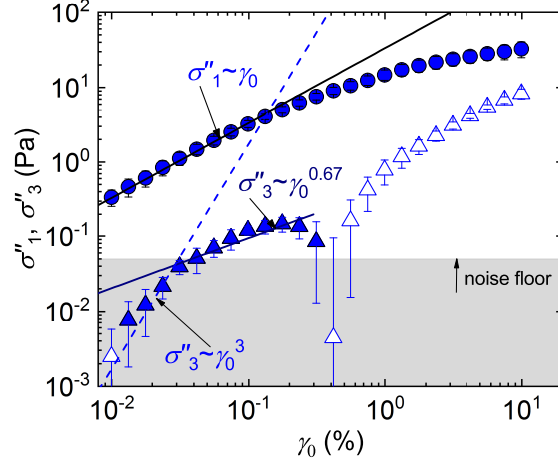

Figure S2: Typical viscous data set for pendular state sample (NP3-silicone oil-glycerol), where  $m_{3,\text{viscous}}$  is less than unity. This sample has a  $\phi_{\text{solid}} = 0.25$  and  $\phi_{2\text{nd}}/\phi_{\text{solid}} = 0.05$ . This data subset is from triplicate sweep measurements at  $\omega = 0.628$  rad/s for the 2<sup>nd</sup> up measurement subset with  $\gamma_{0,\text{max}} = 10\%$ . The filled symbols denote positive values and the empty ones negative values. The gray area refers to the noise floor and was determined using the power spectrum (see Figure S1b). A fitting function with a cubical scaling ( $\sigma_3'' \sim \gamma_0^3$ ) is shown as a reference, which is obscured beneath the noise floor and can only fit few data points with large variances. Thus, this cubical scaling is less trustworthy than the less than unity scaling, for now. However, if the rheometer manufacture can push down the experimental limit in the future (e.g. access to a lower strain or lower minimum torque limit), there might be a chance to claim a cubical scaling with a confidence.

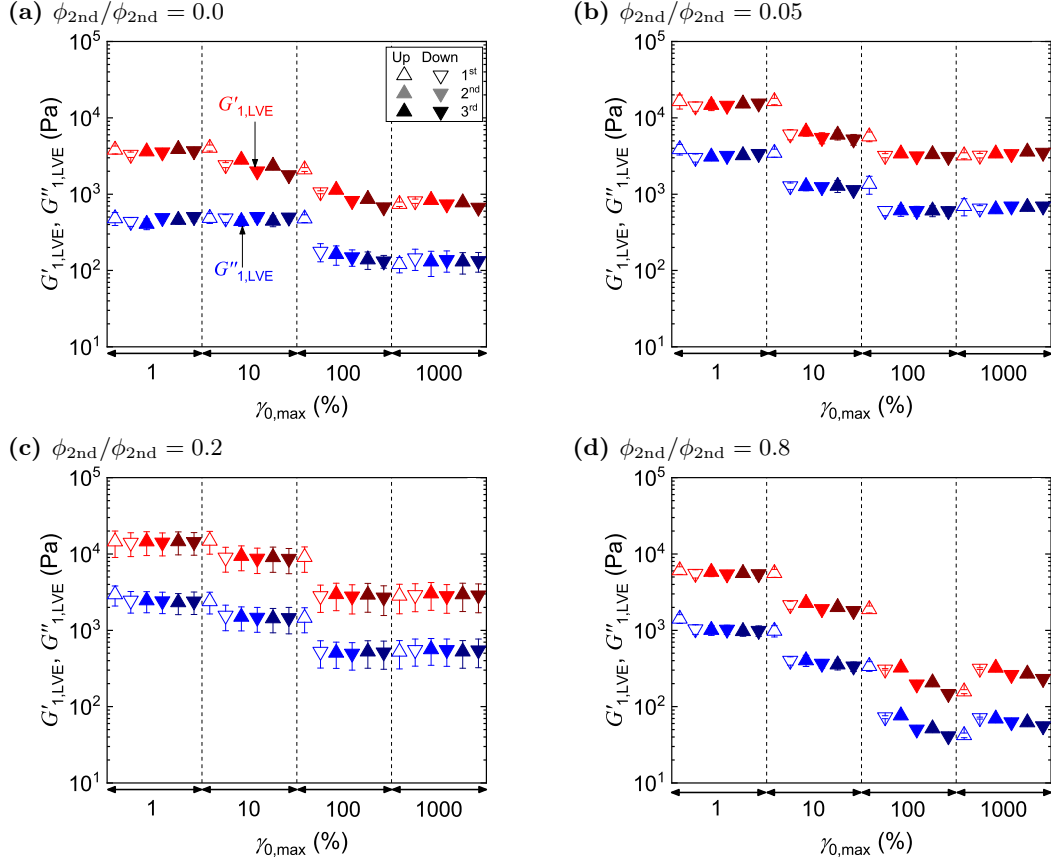

Figure S3: All calculated  $G'_{\text{LVE}}$  (red) and  $G''_{\text{LVE}}$  values (blue) from capillary suspension in the pendular state (NP3-silicone oil-glycerol suspension). Solid concentration is constant  $\phi_{\text{solid}} = 0.25$ . The concentration of secondary fluid is varied as follows: (a)  $\phi_{2\text{nd}}/\phi_{\text{solid}} = 0$ , (b)  $\phi_{2\text{nd}}/\phi_{\text{solid}} = 0.05$ , (c)  $\phi_{2\text{nd}}/\phi_{\text{solid}} = 0.2$ , and (d)  $\phi_{2\text{nd}}/\phi_{\text{solid}} = 0.8$ . Each data point in each subfigure represents the average  $G'_{\text{LVE}}$  and  $G''_{\text{LVE}}$  value from triplicate strain amplitude oscillatory measurements in a range of  $10^{-2} \leq \gamma_0 \leq \gamma_{0,\max}$ .

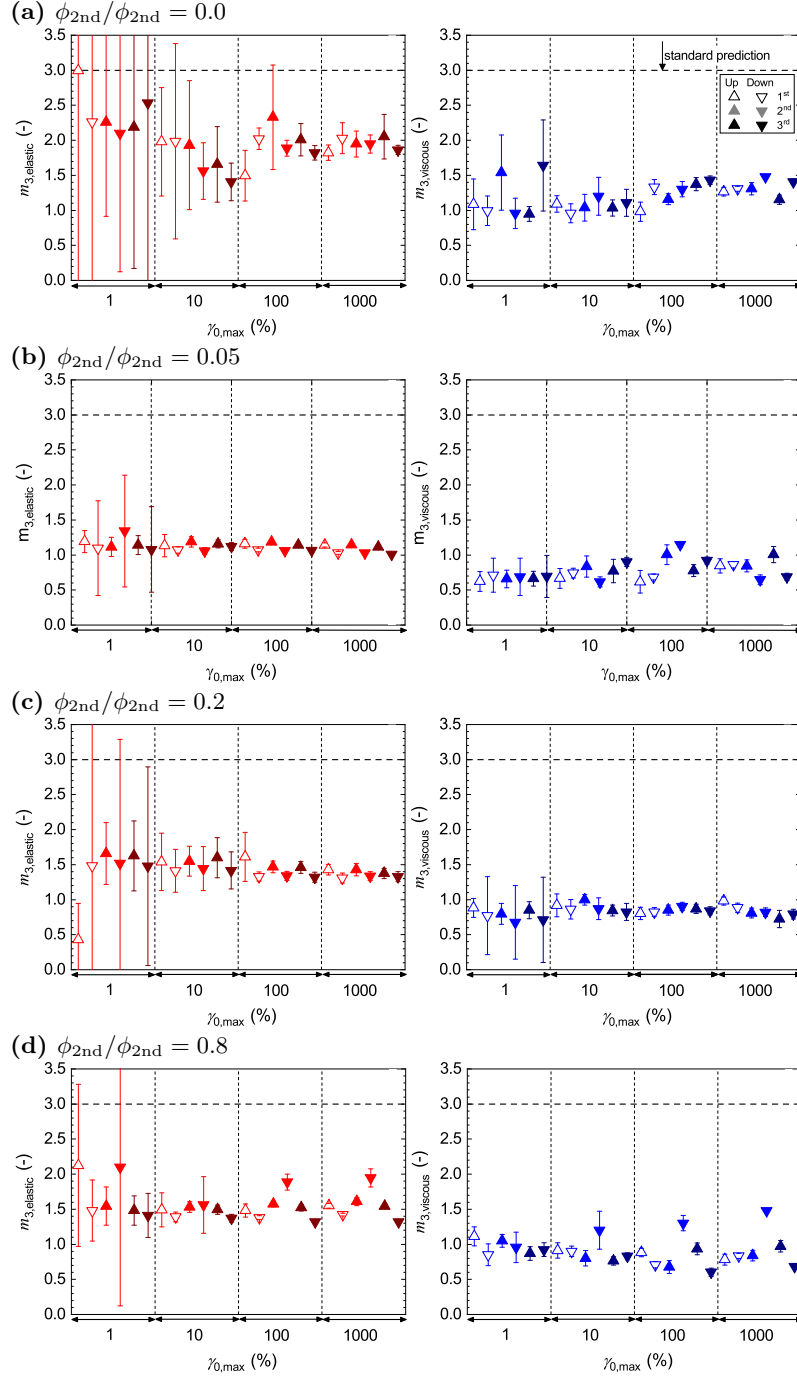

Figure S4: Third harmonic elastic (in red) and viscous (in blue) weakly nonlinear scaling of capillary suspensions in the pendular state with different concentration of secondary fluid.

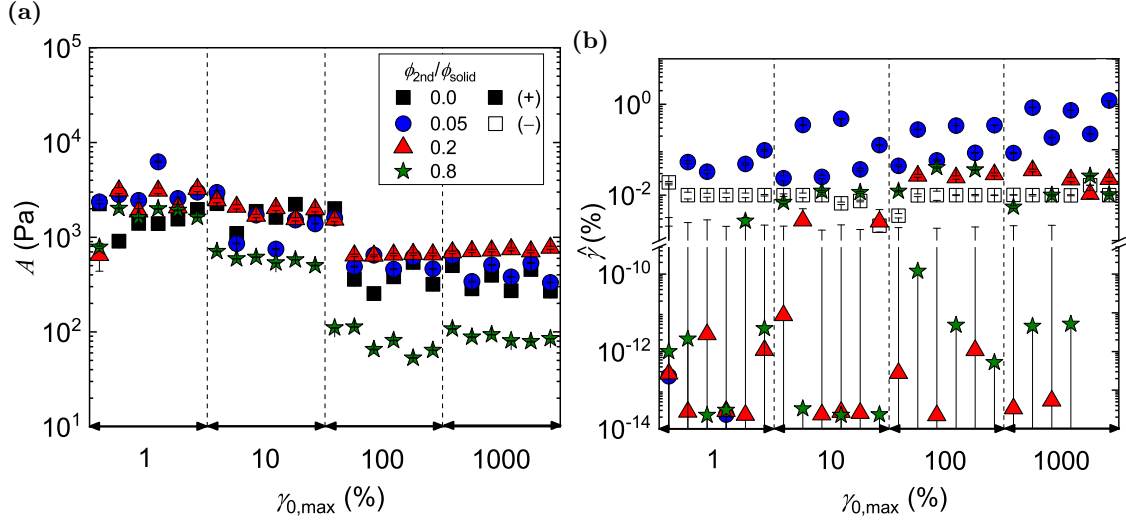

Figure S5: Fitting results from the fitting equation  $-\sigma'_3 \sim A(\gamma_0 + \hat{\gamma})^{3/2} - A\hat{\gamma}^{3/2}$  for NP3 in silicone oil with added glycerol samples, where (a)  $A$  and (b)  $\hat{\gamma}$ .  $0.0 \leq \phi_{solid} \leq 0.8$  with different concentration of secondary fluid.

Table S1: Obtained values for the fitting parameters  $A$  and  $\hat{\gamma}$  for samples in the pendular state.

| $\phi_{2\text{nd}}/\phi_{\text{solid}}$ | $\gamma_{0,\text{max}}$ | step | $A$ [Pa]        |                 | $\hat{\gamma}$ [%]    |                      |
|-----------------------------------------|-------------------------|------|-----------------|-----------------|-----------------------|----------------------|
|                                         |                         |      | up              | down            | up                    | down                 |
| 0                                       | 1%                      | 1    | 2250 $\pm$ 50   | 910 $\pm$ 50    | -0.0191 $\pm$ 0.0008  | -0.010 $\pm$ 0.002   |
|                                         |                         | 2    | 1400 $\pm$ 40   | 1400 $\pm$ 40   | -0.010 $\pm$ 0.001    | -0.010 $\pm$ 0.001   |
|                                         |                         | 3    | 1550 $\pm$ 50   | 1960 $\pm$ 30   | -0.010 $\pm$ 0.001    | -0.0100 $\pm$ 0.0004 |
|                                         | 10%                     | 1    | 2260 $\pm$ 50   | 1100 $\pm$ 40   | -0.0100 $\pm$ 0.0006  | -0.010 $\pm$ 0.001   |
|                                         |                         | 2    | 1870 $\pm$ 30   | 1620 $\pm$ 10   | -0.0100 $\pm$ 0.0005  | -0.0066 $\pm$ 0.0004 |
|                                         |                         | 3    | 2230 $\pm$ 20   | 1530 $\pm$ 10   | -0.0075 $\pm$ 0.0003  | -0.0021 $\pm$ 0.0006 |
|                                         | 100%                    | 1    | 2010 $\pm$ 10   | 359 $\pm$ 6     | -0.0035 $\pm$ 0.0004  | -0.0099 $\pm$ 0.0007 |
|                                         |                         | 2    | 260 $\pm$ 20    | 382.3 $\pm$ 0.9 | -0.010 $\pm$ 0.002    | -0.0100 $\pm$ 0.0002 |
|                                         |                         | 3    | 541 $\pm$ 2     | 318.9 $\pm$ 0.6 | -0.0100 $\pm$ 0.0003  | -0.0100 $\pm$ 0.0002 |
|                                         | 1000%                   | 1    | 500.5 $\pm$ 0.4 | 286 $\pm$ 2     | -0.01009 $\pm$ 0.0001 | -0.0100 $\pm$ 0.0004 |
|                                         |                         | 2    | 397 $\pm$ 3     | 272.7 $\pm$ 0.7 | -0.0100 $\pm$ 0.0004  | -0.0099 $\pm$ 0.0002 |
|                                         |                         | 3    | 456 $\pm$ 1     | 269 $\pm$ 0.4   | -0.0165 $\pm$ 0.0002  | -0.0100 $\pm$ 0.0002 |
| 0.05                                    | 1%                      | 1    | 2400 $\pm$ 100  | 2800 $\pm$ 200  | 2.3E-13 $\pm$ 0.003   | 0.053 $\pm$ 0.004    |
|                                         |                         | 2    | 2400 $\pm$ 100  | 6200 $\pm$ 100  | 0.033 $\pm$ 0.003     | 2.3E-14 $\pm$ 0.0006 |
|                                         |                         | 3    | 2600 $\pm$ 100  | 3000 $\pm$ 100  | 0.049 $\pm$ 0.003     | 0.097 $\pm$ 0.004    |
|                                         | 10%                     | 1    | 3000 $\pm$ 100  | 860 $\pm$ 10    | 0.024 $\pm$ 0.003     | 0.352 $\pm$ 0.004    |
|                                         |                         | 2    | 1710 $\pm$ 50   | 750 $\pm$ 10    | 0.025 $\pm$ 0.002     | 0.479 $\pm$ 0.005    |
|                                         |                         | 3    | 1520 $\pm$ 40   | 1390 $\pm$ 10   | 0.037 $\pm$ 0.002     | 0.127 $\pm$ 0.001    |
|                                         | 100%                    | 1    | 1590 $\pm$ 40   | 489 $\pm$ 5     | 0.044 $\pm$ 0.002     | 0.277 $\pm$ 0.003    |
|                                         |                         | 2    | 646 $\pm$ 9     | 459 $\pm$ 5     | 0.058 $\pm$ 0.002     | 0.341 $\pm$ 0.003    |
|                                         |                         | 3    | 617 $\pm$ 9     | 463 $\pm$ 5     | 0.085 $\pm$ 0.002     | 0.344 $\pm$ 0.003    |
|                                         | 1000%                   | 1    | 637 $\pm$ 10    | 340 $\pm$ 2     | 0.084 $\pm$ 0.002     | 0.847 $\pm$ 0.004    |
|                                         |                         | 2    | 509 $\pm$ 4     | 381 $\pm$ 3     | 0.185 $\pm$ 0.002     | 0.737 $\pm$ 0.004    |
|                                         |                         | 3    | 534 $\pm$ 5     | 332 $\pm$ 2     | 0.221 $\pm$ 0.002     | 1.205 $\pm$ 0.006    |
| 0.2                                     | 1%                      | 1    | 600 $\pm$ 200   | 3100 $\pm$ 200  | 2.6E-13 $\pm$ 0.02    | 2.7E-14 $\pm$ 0.002  |
|                                         |                         | 2    | 1900 $\pm$ 100  | 3100 $\pm$ 200  | 2.8E-12 $\pm$ 0.003   | 2.9E-14 $\pm$ 0.002  |
|                                         |                         | 3    | 2100 $\pm$ 100  | 3200 $\pm$ 200  | 2.3E-14 $\pm$ 0.003   | 1.1E-12 $\pm$ 0.002  |
|                                         | 10%                     | 1    | 2400 $\pm$ 100  | 2100 $\pm$ 100  | 8.6E-12 $\pm$ 0.002   | 0.003 $\pm$ 0.002    |
|                                         |                         | 2    | 1680 $\pm$ 60   | 2000 $\pm$ 100  | 2.3E-14 $\pm$ 0.002   | 2.7E-14 $\pm$ 0.002  |
|                                         |                         | 3    | 1550 $\pm$ 60   | 2000 $\pm$ 100  | 2.5E-14 $\pm$ 0.002   | 0.003 $\pm$ 0.002    |
|                                         | 100%                    | 1    | 1530 $\pm$ 70   | 640 $\pm$ 20    | 2.7E-13 $\pm$ 0.002   | 0.027 $\pm$ 0.002    |
|                                         |                         | 2    | 640 $\pm$ 20    | 660 $\pm$ 20    | 2.2E-14 $\pm$ 0.002   | 0.024 $\pm$ 0.002    |
|                                         |                         | 3    | 660 $\pm$ 20    | 660 $\pm$ 20    | 1.1E-12 $\pm$ 0.002   | 0.029 $\pm$ 0.002    |
|                                         | 1000%                   | 1    | 690 $\pm$ 20    | 710 $\pm$ 20    | 3.3E-14 $\pm$ 0.002   | 0.035 $\pm$ 0.002    |
|                                         |                         | 2    | 720 $\pm$ 20    | 740 $\pm$ 30    | 5.3E-14 $\pm$ 0.002   | 0.022 $\pm$ 0.002    |
|                                         |                         | 3    | 710 $\pm$ 20    | 770 $\pm$ 30    | 0.011 $\pm$ 0.002     | 0.022 $\pm$ 0.002    |
| 0.8                                     | 1%                      | 1    | 780 $\pm$ 20    | 2020 $\pm$ 20   | 9.9E-13 $\pm$ 0.002   | 2.1E-12 $\pm$ 0.0005 |
|                                         |                         | 2    | 1610 $\pm$ 10   | 2000 $\pm$ 20   | 2.2E-14 $\pm$ 0.0005  | 3.1E-14 $\pm$ 0.0006 |
|                                         |                         | 3    | 1920 $\pm$ 20   | 1620 $\pm$ 20   | 0.0027 $\pm$ 0.0005   | 3.9E-12 $\pm$ 0.0005 |
|                                         | 10%                     | 1    | 709 $\pm$ 4     | 593 $\pm$ 3     | 0.007 $\pm$ 0.0005    | 3.3E-14 $\pm$ 0.0004 |
|                                         |                         | 2    | 615 $\pm$ 4     | 535 $\pm$ 2     | 0.0122 $\pm$ 0.0006   | 2.2E-14 $\pm$ 0.0004 |
|                                         |                         | 3    | 578 $\pm$ 4     | 502 $\pm$ 3     | 0.0115 $\pm$ 0.0006   | 2.3E-14 $\pm$ 0.0006 |
|                                         | 100%                    | 1    | 110.3 $\pm$ 0.5 | 112.9 $\pm$ 0.4 | 0.0123 $\pm$ 0.0005   | 1.2E-10 $\pm$ 0.0004 |
|                                         |                         | 2    | 65.3 $\pm$ 0.5  | 81.2 $\pm$ 0.3  | 0.041 $\pm$ 0.001     | 4.8E-12 $\pm$ 0.0004 |
|                                         |                         | 3    | 53.1 $\pm$ 0.4  | 64.1 $\pm$ 0.2  | 0.036 $\pm$ 0.001     | 5.2E-13 $\pm$ 0.0003 |
|                                         | 1000%                   | 1    | 107.7 $\pm$ 0.3 | 88.4 $\pm$ 0.4  | 0.0055 $\pm$ 0.0003   | 4.5E-12 $\pm$ 0.0005 |
|                                         |                         | 2    | 93.6 $\pm$ 0.4  | 80.7 $\pm$ 0.2  | 0.0100 $\pm$ 0.0004   | 5.1E-12 $\pm$ 0.0003 |
|                                         |                         | 3    | 79 $\pm$ 0.6    | 85 $\pm$ 0.4    | 0.0264 $\pm$ 0.0009   | 0.0103 $\pm$ 0.0005  |

## Capillary state

Table S2: Ratio of viscous scaling to the elastic scaling showing the average and deviation

| State     | $\phi_{2nd}/\phi_{solid}$ | $\frac{m_{3,viscous}}{m_{3,elastic}}, average$ | $\delta \frac{m_{3,viscous}}{m_{3,elastic}}$ |
|-----------|---------------------------|------------------------------------------------|----------------------------------------------|
| pendular  | 0.0                       | 0.71                                           | 0.01                                         |
|           | 0.05                      | 0.76                                           | 0.03                                         |
|           | 0.2                       | 0.61                                           | 0.01                                         |
|           | 0.8                       | 0.54                                           | 0.01                                         |
| capillary | 0.0                       | 0.97                                           | 0.03                                         |
|           | 0.1                       | 0.74                                           | 0.02                                         |
|           | 0.2                       | 0.69                                           | 0.01                                         |
|           | 0.3                       | 0.75                                           | 0.01                                         |
|           | 0.8                       | 0.69                                           | 0.02                                         |

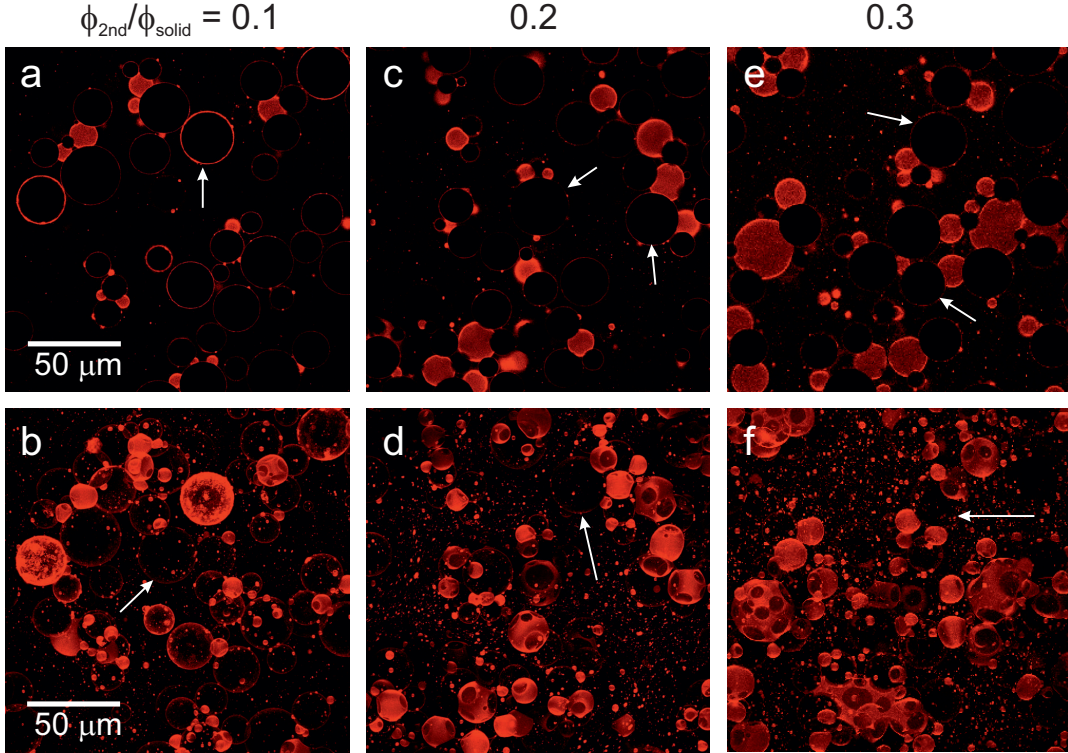

Figure S6: Confocal microscope images with (a,b)  $\phi_{2nd}/\phi_{solid} = 0.1$ , (c,d)  $\phi_{2nd}/\phi_{solid} = 0.2$ , (e,f)  $\phi_{2nd}/\phi_{solid} = 0.3$ . The upper images show a 2D-image slice and the lower images the image of 3D stack. Paraffin oil, the secondary fluid, is dyed with Nile red and appear as red droplets. The intensity of the images is enhanced, so PMMA particles ( $\phi_{solid} = 0.25$ ) have a better visibility (shown as a red ring. See the example particles, denoted by arrows, in each image.).

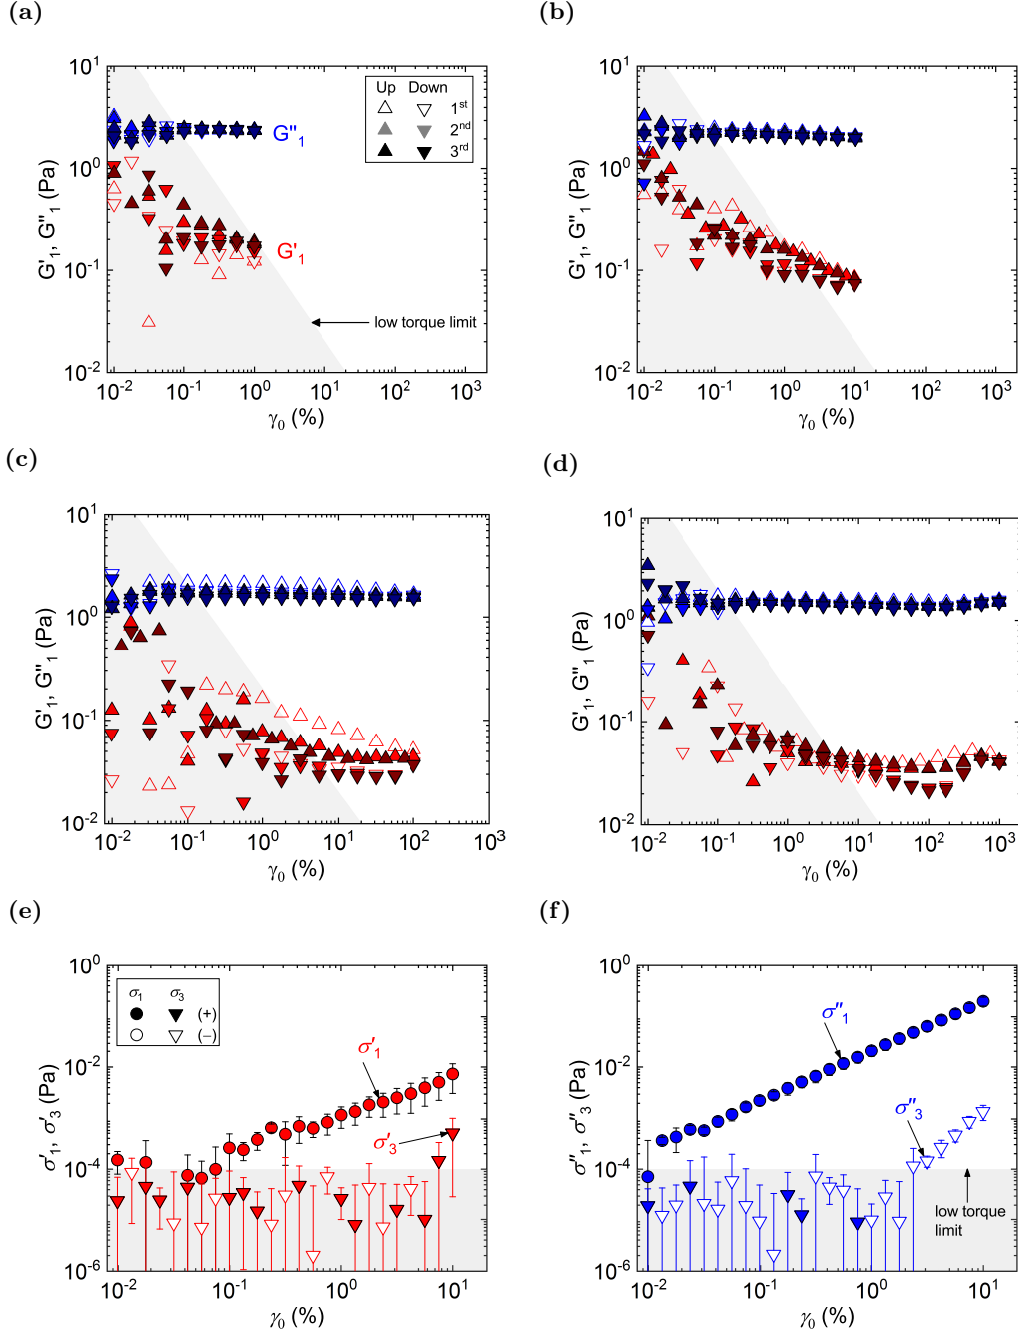

Figure S7:  $G'$  and  $G''$  from PMMA-glycerol normal suspension from three consecutive strain-amplitude sweeps in increasing (up triangle) and decreasing (down triangle) amplitude. Four maximum amplitudes ( $\gamma_{0,\max} = 1\%$  (a),  $10\%$  (b),  $100\%$  (c), and  $1000\%$  (d)) were run in succession using the same sample. The gray area represents the experimental limit corresponding to the 50 nNm torque limit given by manufacturer. (e) Limited data points above the noise floor for the elastic third harmonic stress analysis for  $\gamma_{0,\max} \leq 10\%$ . Therefore only data set with  $\gamma_{0,\max} \geq 100\%$  are used for further analysis. (f) The viscous third harmonic stress signal for  $\gamma_{0,\max} \geq 1\%$  raises above the noise floor. Thus,  $\gamma_{0,\max} = 1\%$  is set as the lower limit for third harmonic viscous stress analysis for PMMA-glycerol normal suspension.

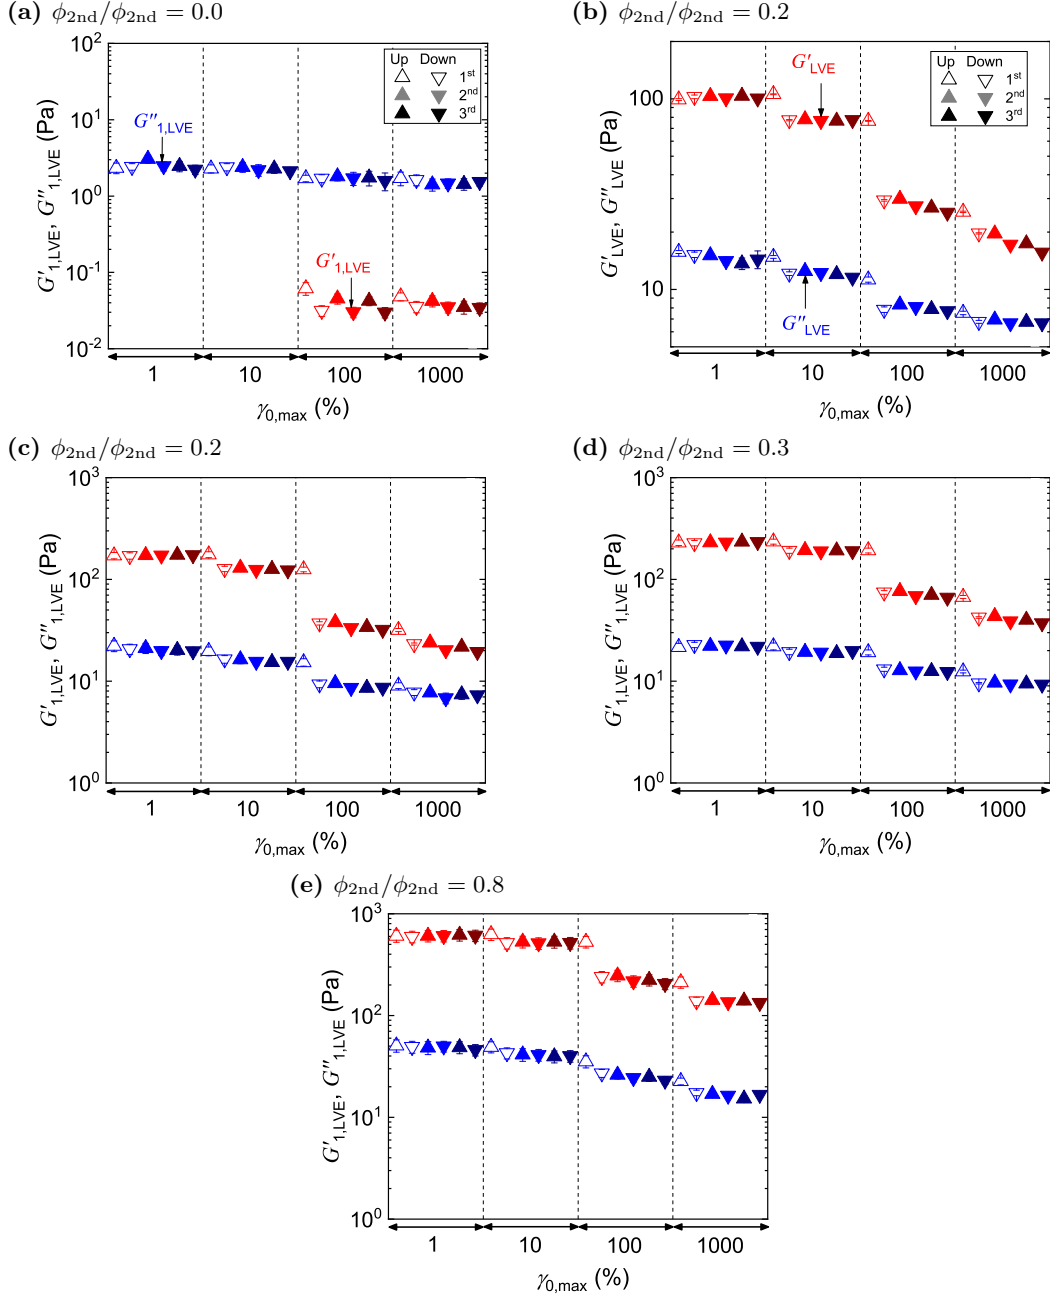

Figure S8: All calculated  $G'_{\text{LVE}}$  (red) and  $G''_{\text{LVE}}$  values (blue) from capillary suspension in the capillary state (PMMA-glycerol-paraffin oil suspensions). Solid concentration is constant  $\phi_{\text{solid}} = 0.25$ . The concentration of secondary fluid is varied as follows: (a)  $\phi_{2\text{nd}}/\phi_{\text{solid}} = 0$ , (b)  $\phi_{2\text{nd}}/\phi_{\text{solid}} = 0.1$ , (c)  $\phi_{2\text{nd}}/\phi_{\text{solid}} = 0.2$ , (d)  $\phi_{2\text{nd}}/\phi_{\text{solid}} = 0.2$ , and (e)  $\phi_{2\text{nd}}/\phi_{\text{solid}} = 0.8$ . Each data point in each subfigure represents the average  $G'_{\text{LVE}}$  and  $G''_{\text{LVE}}$  value from triplicate strain amplitude oscillatory measurements in a range of  $10^{-2} \leq \gamma_0 \leq \gamma_{0,\text{max}}$ .

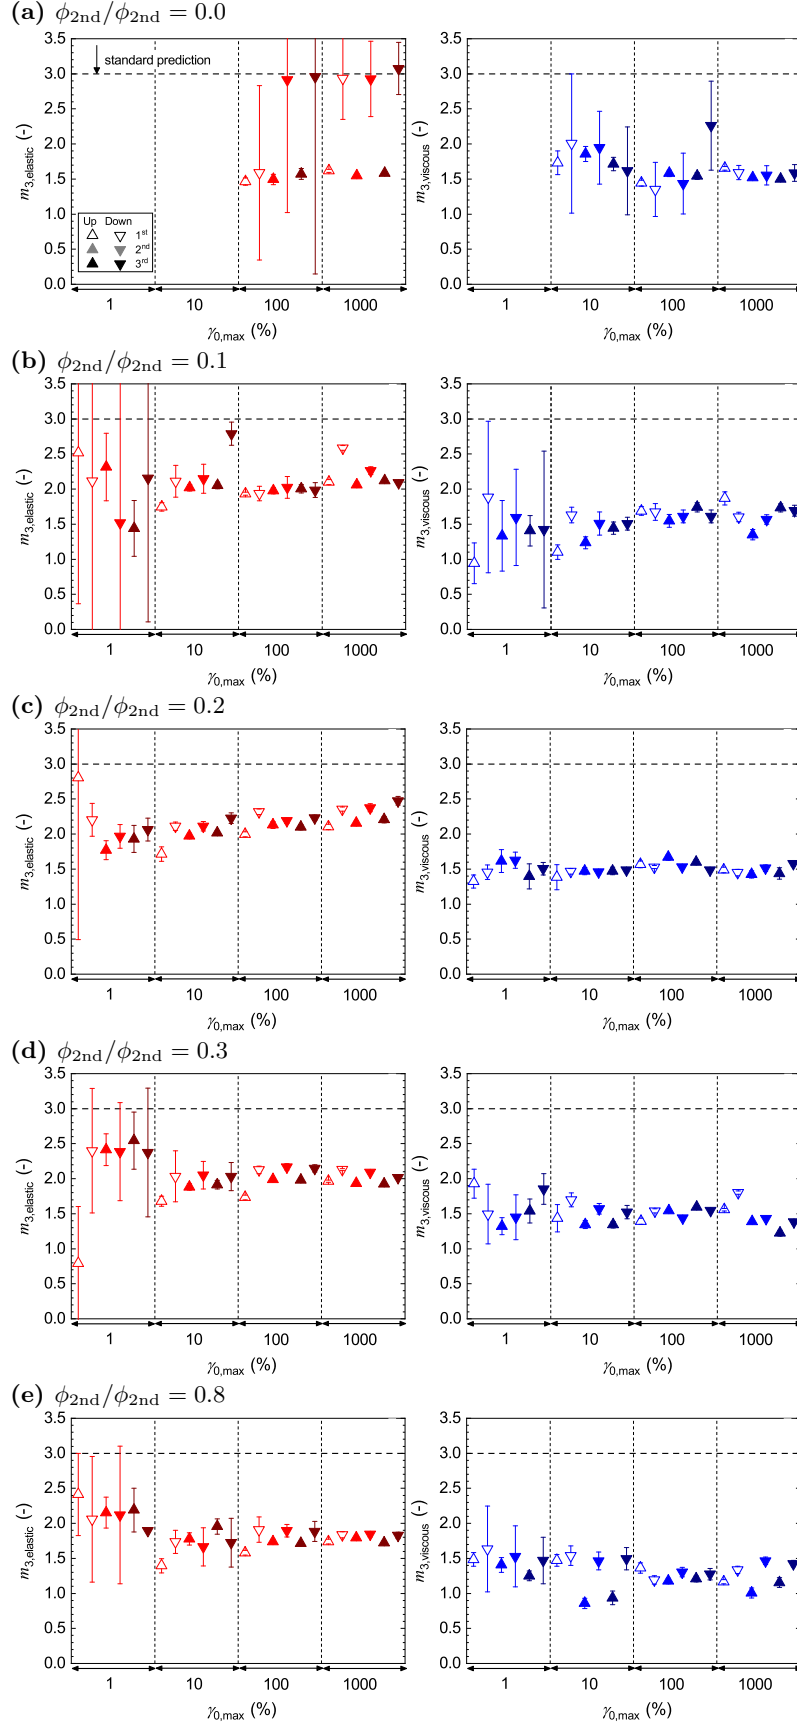

Figure S9: Third harmonic elastic (in red) and viscous (in blue) weakly nonlinear scaling of capillary suspensions in the capillary state with different concentration of secondary fluid.

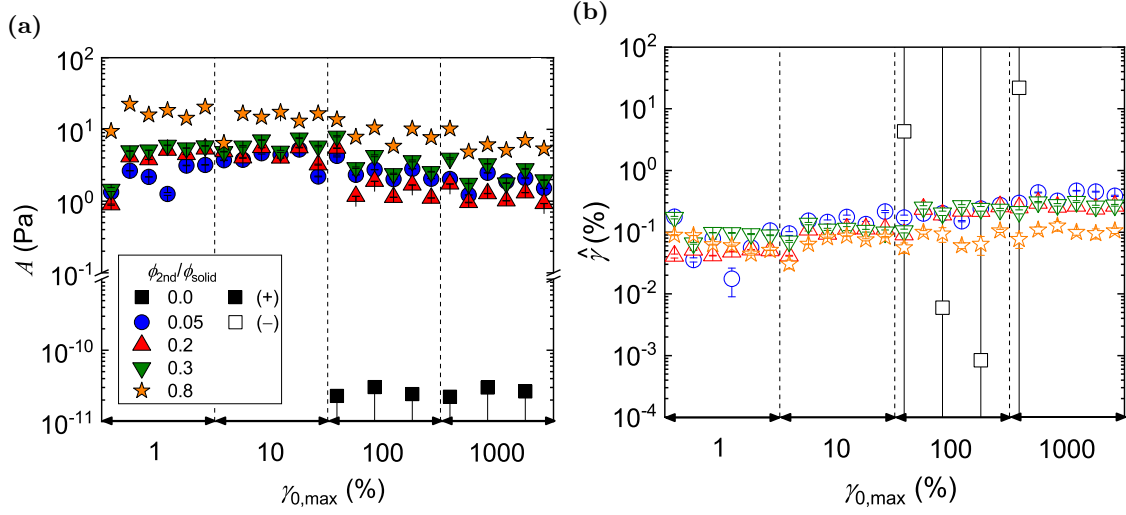

Figure S10: Fitting results from the fitting equation 15 for PMMA in glycerol with added paraffin oil samples, where (a)  $A$ , and (b)  $\hat{\gamma}$ .  $0.0 \leq \phi_{2\text{nd}}/\phi_{\text{solid}} \leq 0.8$ . with different concentration of secondary fluid. Hollow symbols denote negative values of  $\hat{\gamma}$  and refer to strain needed to bring the particles into contact.

Table S3: Obtained values for the fitting parameters  $A$  and  $\hat{\gamma}$  for samples in the capillary state.

| $\phi_{2nd}/\phi_{solid}$ | $\gamma_{0,max}$ | step | $A$ [Pa]             |                   | $\hat{\gamma}$ [%]      |                      |
|---------------------------|------------------|------|----------------------|-------------------|-------------------------|----------------------|
|                           |                  |      | up                   | down              | up                      | down                 |
| 0                         | 1%               | 1    | -                    | -                 | -                       | -                    |
|                           |                  | 2    | -                    | -                 | -                       | -                    |
|                           |                  | 3    | -                    | -                 | -                       | -                    |
|                           | 10%              | 1    | -                    | -                 | -                       | -                    |
|                           |                  | 2    | -                    | -                 | -                       | -                    |
|                           |                  | 3    | -                    | -                 | -                       | -                    |
|                           | 100%             | 1    | $2.3E-11 \pm 0.0008$ | -                 | $-4.3 \pm 3.00E+08$     | -                    |
|                           |                  | 2    | $3.0E-11 \pm 0.0001$ | -                 | $-0.0060 \pm 3.00E+07$  | -                    |
|                           |                  | 3    | $2.4E-11 \pm 0.0001$ | -                 | $-0.0008 \pm 3.00E+07$  | -                    |
|                           | 1000%            | 1    | $2.2E-11 \pm 0.001$  | -                 | $-21.9 \pm 3.00E+09$    | -                    |
|                           |                  | 2    | $3.0E-11 \pm 0.0003$ | -                 | $-1.2E-06 \pm 1.00E+08$ | -                    |
|                           |                  | 3    | $2.6E-11 \pm 0.0003$ | -                 | $-1.6E-06 \pm 1.00E+08$ | -                    |
| 0.1                       | 1%               | 1    | $1.3 \pm 0.1$        | $2.65 \pm 0.02$   | $-0.18 \pm 0.02$        | $-0.036 \pm 0.003$   |
|                           |                  | 2    | $2.17 \pm 0.02$      | $1.26 \pm 0.06$   | $-0.079 \pm 0.002$      | $-0.018 \pm 0.009$   |
|                           |                  | 3    | $3.13 \pm 0.03$      | $3.20 \pm 0.03$   | $-0.056 \pm 0.003$      | $-0.106 \pm 0.003$   |
|                           | 10%              | 1    | $3.71 \pm 0.04$      | $3.75 \pm 0.06$   | $-0.095 \pm 0.007$      | $-0.15 \pm 0.01$     |
|                           |                  | 2    | $4.6 \pm 0.1$        | $4.44 \pm 0.07$   | $-0.15 \pm 0.01$        | $-0.18 \pm 0.01$     |
|                           |                  | 3    | $5.2 \pm 0.1$        | $2.21 \pm 0.03$   | $-0.14 \pm 0.01$        | $-0.216 \pm 0.009$   |
|                           | 100%             | 1    | $4.3 \pm 0.1$        | $2.327 \pm 0.004$ | $-0.17 \pm 0.02$        | $-0.202 \pm 0.005$   |
|                           |                  | 2    | $2.74 \pm 0.01$      | $2.028 \pm 0.004$ | $-0.203 \pm 0.006$      | $-0.151 \pm 0.004$   |
|                           |                  | 3    | $2.818 \pm 0.007$    | $2.055 \pm 0.002$ | $-0.242 \pm 0.004$      | $-0.276 \pm 0.003$   |
|                           | 1000%            | 1    | $2.04 \pm 0.02$      | $1.215 \pm 0.005$ | $-0.298 \pm 0.009$      | $-0.44 \pm 0.007$    |
|                           |                  | 2    | $2.476 \pm 0.008$    | $1.881 \pm 0.002$ | $-0.321 \pm 0.006$      | $-0.47 \pm 0.004$    |
|                           |                  | 3    | $2.095 \pm 0.007$    | $1.507 \pm 0.004$ | $-0.455 \pm 0.006$      | $-0.389 \pm 0.009$   |
| 0.2                       | 1%               | 1    | $0.89 \pm 0.02$      | $4.16 \pm 0.03$   | $-0.041 \pm 0.003$      | $-0.052 \pm 0.001$   |
|                           |                  | 2    | $3.802 \pm 0.008$    | $5.14 \pm 0.02$   | $-0.0418 \pm 0.0005$    | $-0.0483 \pm 0.0007$ |
|                           |                  | 3    | $4.461 \pm 0.008$    | $5.33 \pm 0.02$   | $-0.0519 \pm 0.0005$    | $-0.0506 \pm 0.0009$ |
|                           | 10%              | 1    | $4.909 \pm 0.008$    | $4.02 \pm 0.07$   | $-0.0416 \pm 0.0006$    | $-0.110 \pm 0.005$   |
|                           |                  | 2    | $5.59 \pm 0.04$      | $4.00 \pm 0.06$   | $-0.094 \pm 0.003$      | $-0.113 \pm 0.006$   |
|                           |                  | 3    | $5.58 \pm 0.05$      | $3.22 \pm 0.05$   | $-0.114 \pm 0.003$      | $-0.112 \pm 0.005$   |
|                           | 100%             | 1    | $5.47 \pm 0.05$      | $1.165 \pm 0.007$ | $-0.091 \pm 0.004$      | $-0.237 \pm 0.006$   |
|                           |                  | 2    | $1.889 \pm 0.009$    | $1.129 \pm 0.006$ | $-0.192 \pm 0.004$      | $-0.222 \pm 0.005$   |
|                           |                  | 3    | $1.675 \pm 0.008$    | $1.103 \pm 0.005$ | $-0.219 \pm 0.004$      | $-0.261 \pm 0.006$   |
|                           | 1000%            | 1    | $1.737 \pm 0.006$    | $0.956 \pm 0.008$ | $-0.25 \pm 0.004$       | $-0.30 \pm 0.01$     |
|                           |                  | 2    | $1.274 \pm 0.006$    | $1.011 \pm 0.005$ | $-0.257 \pm 0.005$      | $-0.267 \pm 0.006$   |
|                           |                  | 3    | $1.309 \pm 0.005$    | $0.927 \pm 0.003$ | $-0.239 \pm 0.004$      | $-0.266 \pm 0.004$   |
| 0.3                       | 1%               | 1    | $9.38 \pm 0.08$      | $22.48 \pm 0.07$  | $-0.090 \pm 0.001$      | $-0.0881 \pm 0.0003$ |
|                           |                  | 2    | $15.92 \pm 0.08$     | $18.5 \pm 0.2$    | $-0.0629 \pm 0.0008$    | $-0.060 \pm 0.002$   |
|                           |                  | 3    | $14.3 \pm 0.2$       | $20.5 \pm 0.1$    | $-0.044 \pm 0.001$      | $-0.0509 \pm 0.0004$ |
|                           | 10%              | 1    | $6.4 \pm 0.05$       | $16.5 \pm 0.1$    | $-0.03 \pm 0.005$       | $-0.064 \pm 0.001$   |
|                           |                  | 2    | $14.8 \pm 0.2$       | $17.34 \pm 0.04$  | $-0.081 \pm 0.002$      | $-0.0865 \pm 0.0007$ |
|                           |                  | 3    | $13.0 \pm 0.3$       | $16.5 \pm 0.1$    | $-0.075 \pm 0.003$      | $-0.083 \pm 0.002$   |
|                           | 100%             | 1    | $13.7 \pm 0.6$       | $7.8 \pm 0.2$     | $-0.06 \pm 0.01$        | $-0.100 \pm 0.007$   |
|                           |                  | 2    | $10.5 \pm 0.9$       | $5.8 \pm 0.2$     | $-0.09 \pm 0.02$        | $-0.06 \pm 0.006$    |
|                           |                  | 3    | $10.1 \pm 0.9$       | $7.7 \pm 0.2$     | $-0.06 \pm 0.02$        | $-0.105 \pm 0.006$   |
|                           | 1000%            | 1    | $10.1 \pm 0.8$       | $4.8 \pm 0.2$     | $-0.08 \pm 0.02$        | $-0.11 \pm 0.01$     |
|                           |                  | 2    | $6.1 \pm 0.5$        | $5.1 \pm 0.2$     | $-0.13 \pm 0.02$        | $-0.10 \pm 0.01$     |
|                           |                  | 3    | $7.0 \pm 0.3$        | $5.4 \pm 0.1$     | $-0.10 \pm 0.02$        | $-0.11 \pm 0.01$     |
| 0.8                       | 1%               | 1    | $1.45 \pm 0.09$      | $4.99 \pm 0.05$   | $-0.172 \pm 0.008$      | $-0.066 \pm 0.002$   |
|                           |                  | 2    | $5.13 \pm 0.03$      | $6.00 \pm 0.05$   | $-0.098 \pm 0.001$      | $-0.098 \pm 0.002$   |
|                           |                  | 3    | $5.48 \pm 0.05$      | $5.87 \pm 0.05$   | $-0.093 \pm 0.002$      | $-0.089 \pm 0.001$   |
|                           | 10%              | 1    | $4.88 \pm 0.04$      | $5.8 \pm 0.1$     | $-0.071 \pm 0.003$      | $-0.138 \pm 0.006$   |
|                           |                  | 2    | $7.1 \pm 0.09$       | $4.9 \pm 0.2$     | $-0.111 \pm 0.004$      | $-0.115 \pm 0.009$   |
|                           |                  | 3    | $7.5 \pm 0.1$        | $5.8 \pm 0.1$     | $-0.106 \pm 0.005$      | $-0.099 \pm 0.009$   |
|                           | 100%             | 1    | $8.0 \pm 0.2$        | $2.92 \pm 0.07$   | $-0.105 \pm 0.007$      | $-0.25 \pm 0.02$     |
|                           |                  | 2    | $4.3 \pm 0.1$        | $2.4 \pm 0.04$    | $-0.20 \pm 0.02$        | $-0.27 \pm 0.01$     |
|                           |                  | 3    | $3.6 \pm 0.1$        | $2.56 \pm 0.03$   | $-0.24 \pm 0.02$        | $-0.23 \pm 0.01$     |
|                           | 1000%            | 1    | $3.94 \pm 0.09$      | $1.76 \pm 0.01$   | $-0.21 \pm 0.02$        | $-0.307 \pm 0.007$   |
|                           |                  | 2    | $3.31 \pm 0.03$      | $1.78 \pm 0.02$   | $-0.28 \pm 0.01$        | $-0.31 \pm 0.01$     |
|                           |                  | 3    | $2.82 \pm 0.03$      | $1.97 \pm 0.02$   | $-0.26 \pm 0.01$        | $-0.273 \pm 0.008$   |
